# Supplementary material for: Region Embedding with Intra and Inter-View Contrastive Learning
Source: arXiv:2211.08975 source file (2022-11-15)
Supplement: Supplementary file 1 [file appendix.tex]

\clearpage
\section{Appendix}

\subsection{Implementation Details}
In our experiments, we set the embedding dimension $d$ to 32 for all the learning methods following the setting in \cite{zhang2019unifying} for fair comparison. We use the Adaptive Moment Estimation (Adam) optimizer to train the models with a learning rate of 0.001. The weighted parameters $\alpha$ and $\beta$ are set to 0.001 and 1.0 respectively. For the temperature parameter $\tau$, we set it as 0.08 following the study in ~\cite{han2020self}. The negative size for POI view, mobility view, and inter-view contrastive learning are set to 150, 10, and 5 respectively. And the augmentation parameters $p$ and $\delta$ are set to 0.1 and 0.0001 in this study. For all the baseline methods, the learning rate is searched in \{0.0005, 0.001, 0.005, 0.01\}. For MV-PN and CGAL, the hidden layer of AutoEncoder is searched  in \{1, 2, 3\}. For MVURE, we tune the number of heads in multi-head attention among \{4, 8, 16\}.

\subsection{Evaluation Metrics}
NMI, ARI and F-measure are used to evaluate the land usage clustering results in this paper. 
\begin{itemize}
  \item \textbf{Normalized Mutual Information (NMI)} measures the purity of the clustering results, which is defined as
  \begin{equation}
      \text{NMI} = \frac{I(L;C)}{[H(L)+H(C)]/2},
  \end{equation}
  where $L$ is the ground-truth classes and $C$ is the predicted classes. $H(L)$ and $H(C)$ denote the entropy, and $I(L;C)$ denotes the sum of mutual information between the predicted classes and ground-truth classes.
  The score ranges from 0 for worst-case to 1 for perfect matching.
 
  \item \textbf{Adjusted Rand Index (ARI)} calculates the clustering accuracy by viewing the cluster assignments of all pairs of regions as different decisions. It can be defined as 
  \begin{equation}
  \begin{aligned}
      \text{ARI} &= \frac{RI - Expected\_RI}{Max\_RI - Expected\_RI}, \\ 
      \text{RI} &= \frac{TP + TN}{TP + FP + TN + FN},
  \end{aligned}
  \end{equation}
  where $TP/FP$ represents true/false positive and $TN/FN$ denotes true/false negative. For the ARI score, 1 stands for best result and 0 means random labeling.
  
  \item \textbf{F-measure} also views the clustering results of each pair as a series of binary classification decisions, then we can obtain precision, recall based on the predefined $TP/FP$ and $TN/FN$. Then, F-measure is defined as follows. 
  \begin{equation}
    F = \frac{(\lambda^2+1) \cdot Precision \cdot Recall} {\lambda^2 \cdot Precision + Recall}.
  \end{equation}
 We follow the setting in \cite{yao2018representing} and set $\lambda = 0.5$.
\end{itemize}

MAE, RMSE and $R^2$ are used to evaluate the region popularity prediction results in our study.

\begin{itemize}
\item \textbf{Mean Absolute Error (MAE)} measures the average absolute distance between predictions and ground-truths.

\item \textbf{Root Mean Square (RMSE)} measures the average quadratic errors of all predictions.

\item \textbf{Coefficient of Determination ($R^2$)} measures the goodness of fit for regression models, which is defined as %$R^2 = 1 - \sum_{i} (y_i - f_i)^2 / \sum_{i} (y_i - \bar y)^2$,
\begin{equation}
 R^2 = 1 - \frac{ \sum_{i} (y_i - f_i)^2}  { \sum_{i} (y_i - \bar y)^2},
\end{equation}
where $y_i, f_i, \bar y$ are ground truth, model prediction and the mean of ground truth respectively. The larger the $R^2$ is, the better the performance is. 
\end{itemize}

\begin{figure*}[t!]
	\centering
	\setlength{\fboxrule}{0.4pt}
    \setlength{\fboxsep}{0.12cm}
	\begin{subfigure}[b]{0.13\textwidth}
		\fbox{\includegraphics[width=\textwidth]{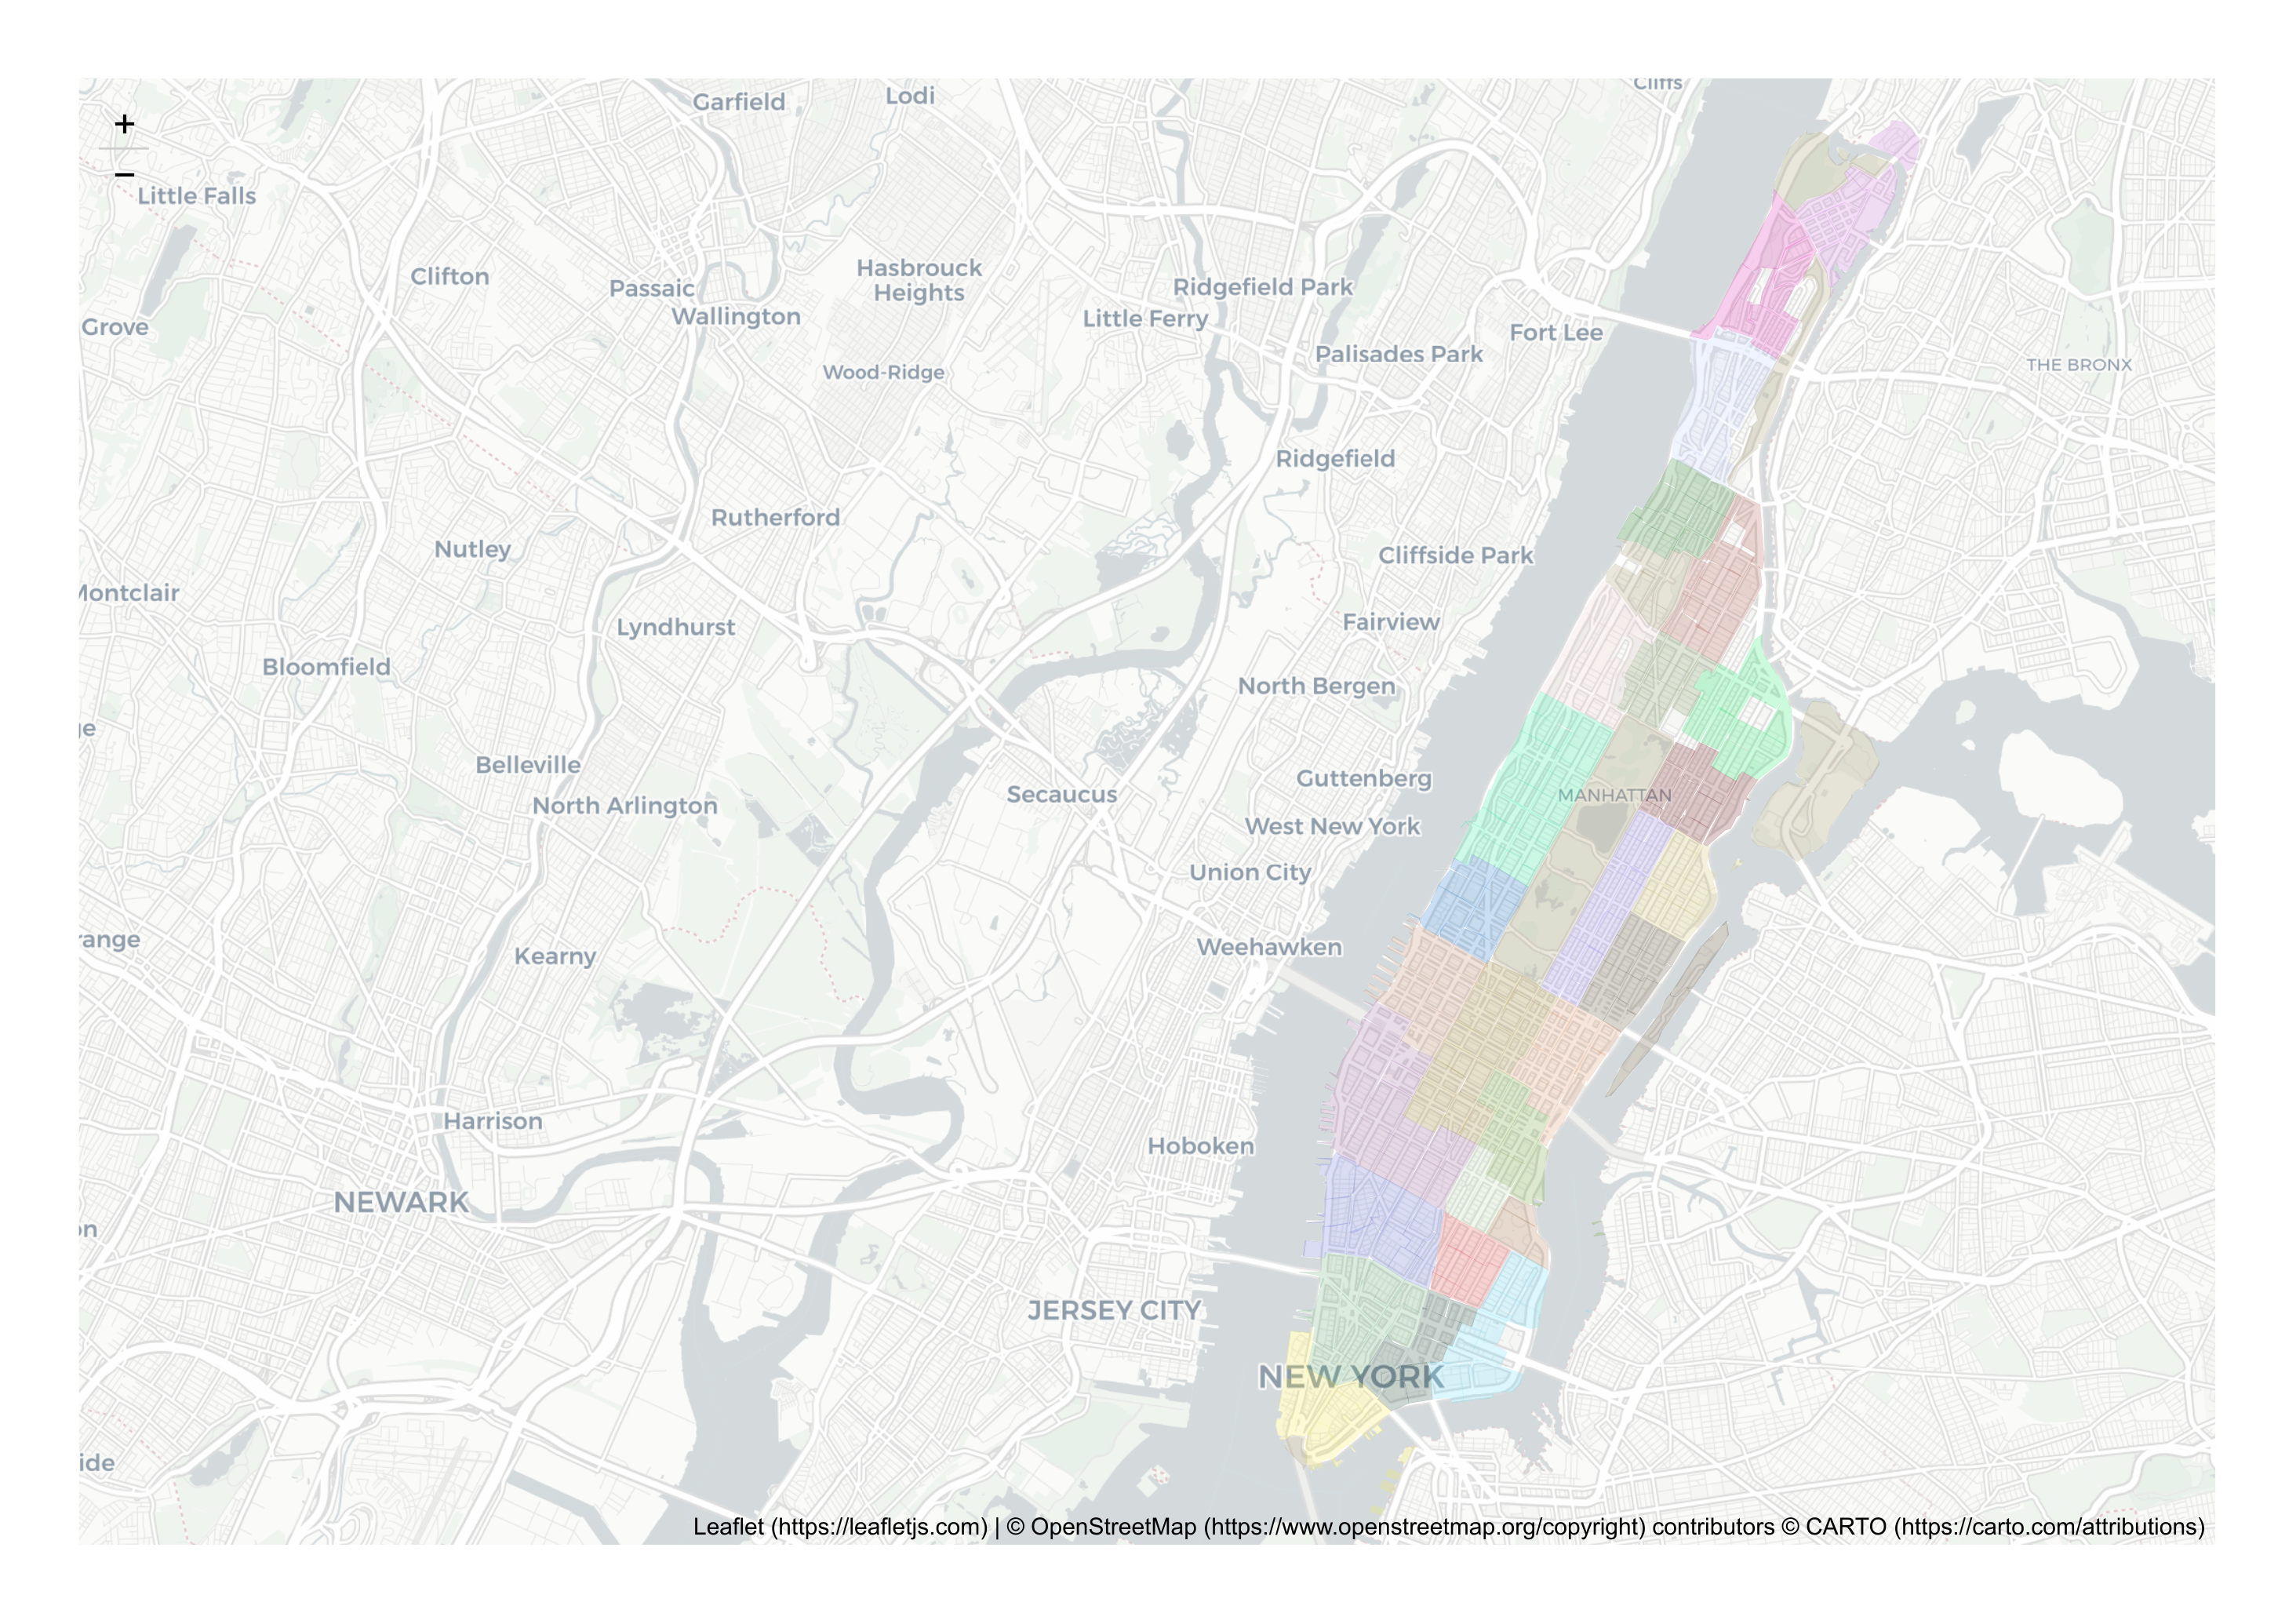}}
		\caption{Labels}
		\label{fig:labels}
	\end{subfigure}
	\hspace{0.02\textwidth}
	\begin{subfigure}[b]{0.13\textwidth}
		\fbox{\includegraphics[width=\textwidth]{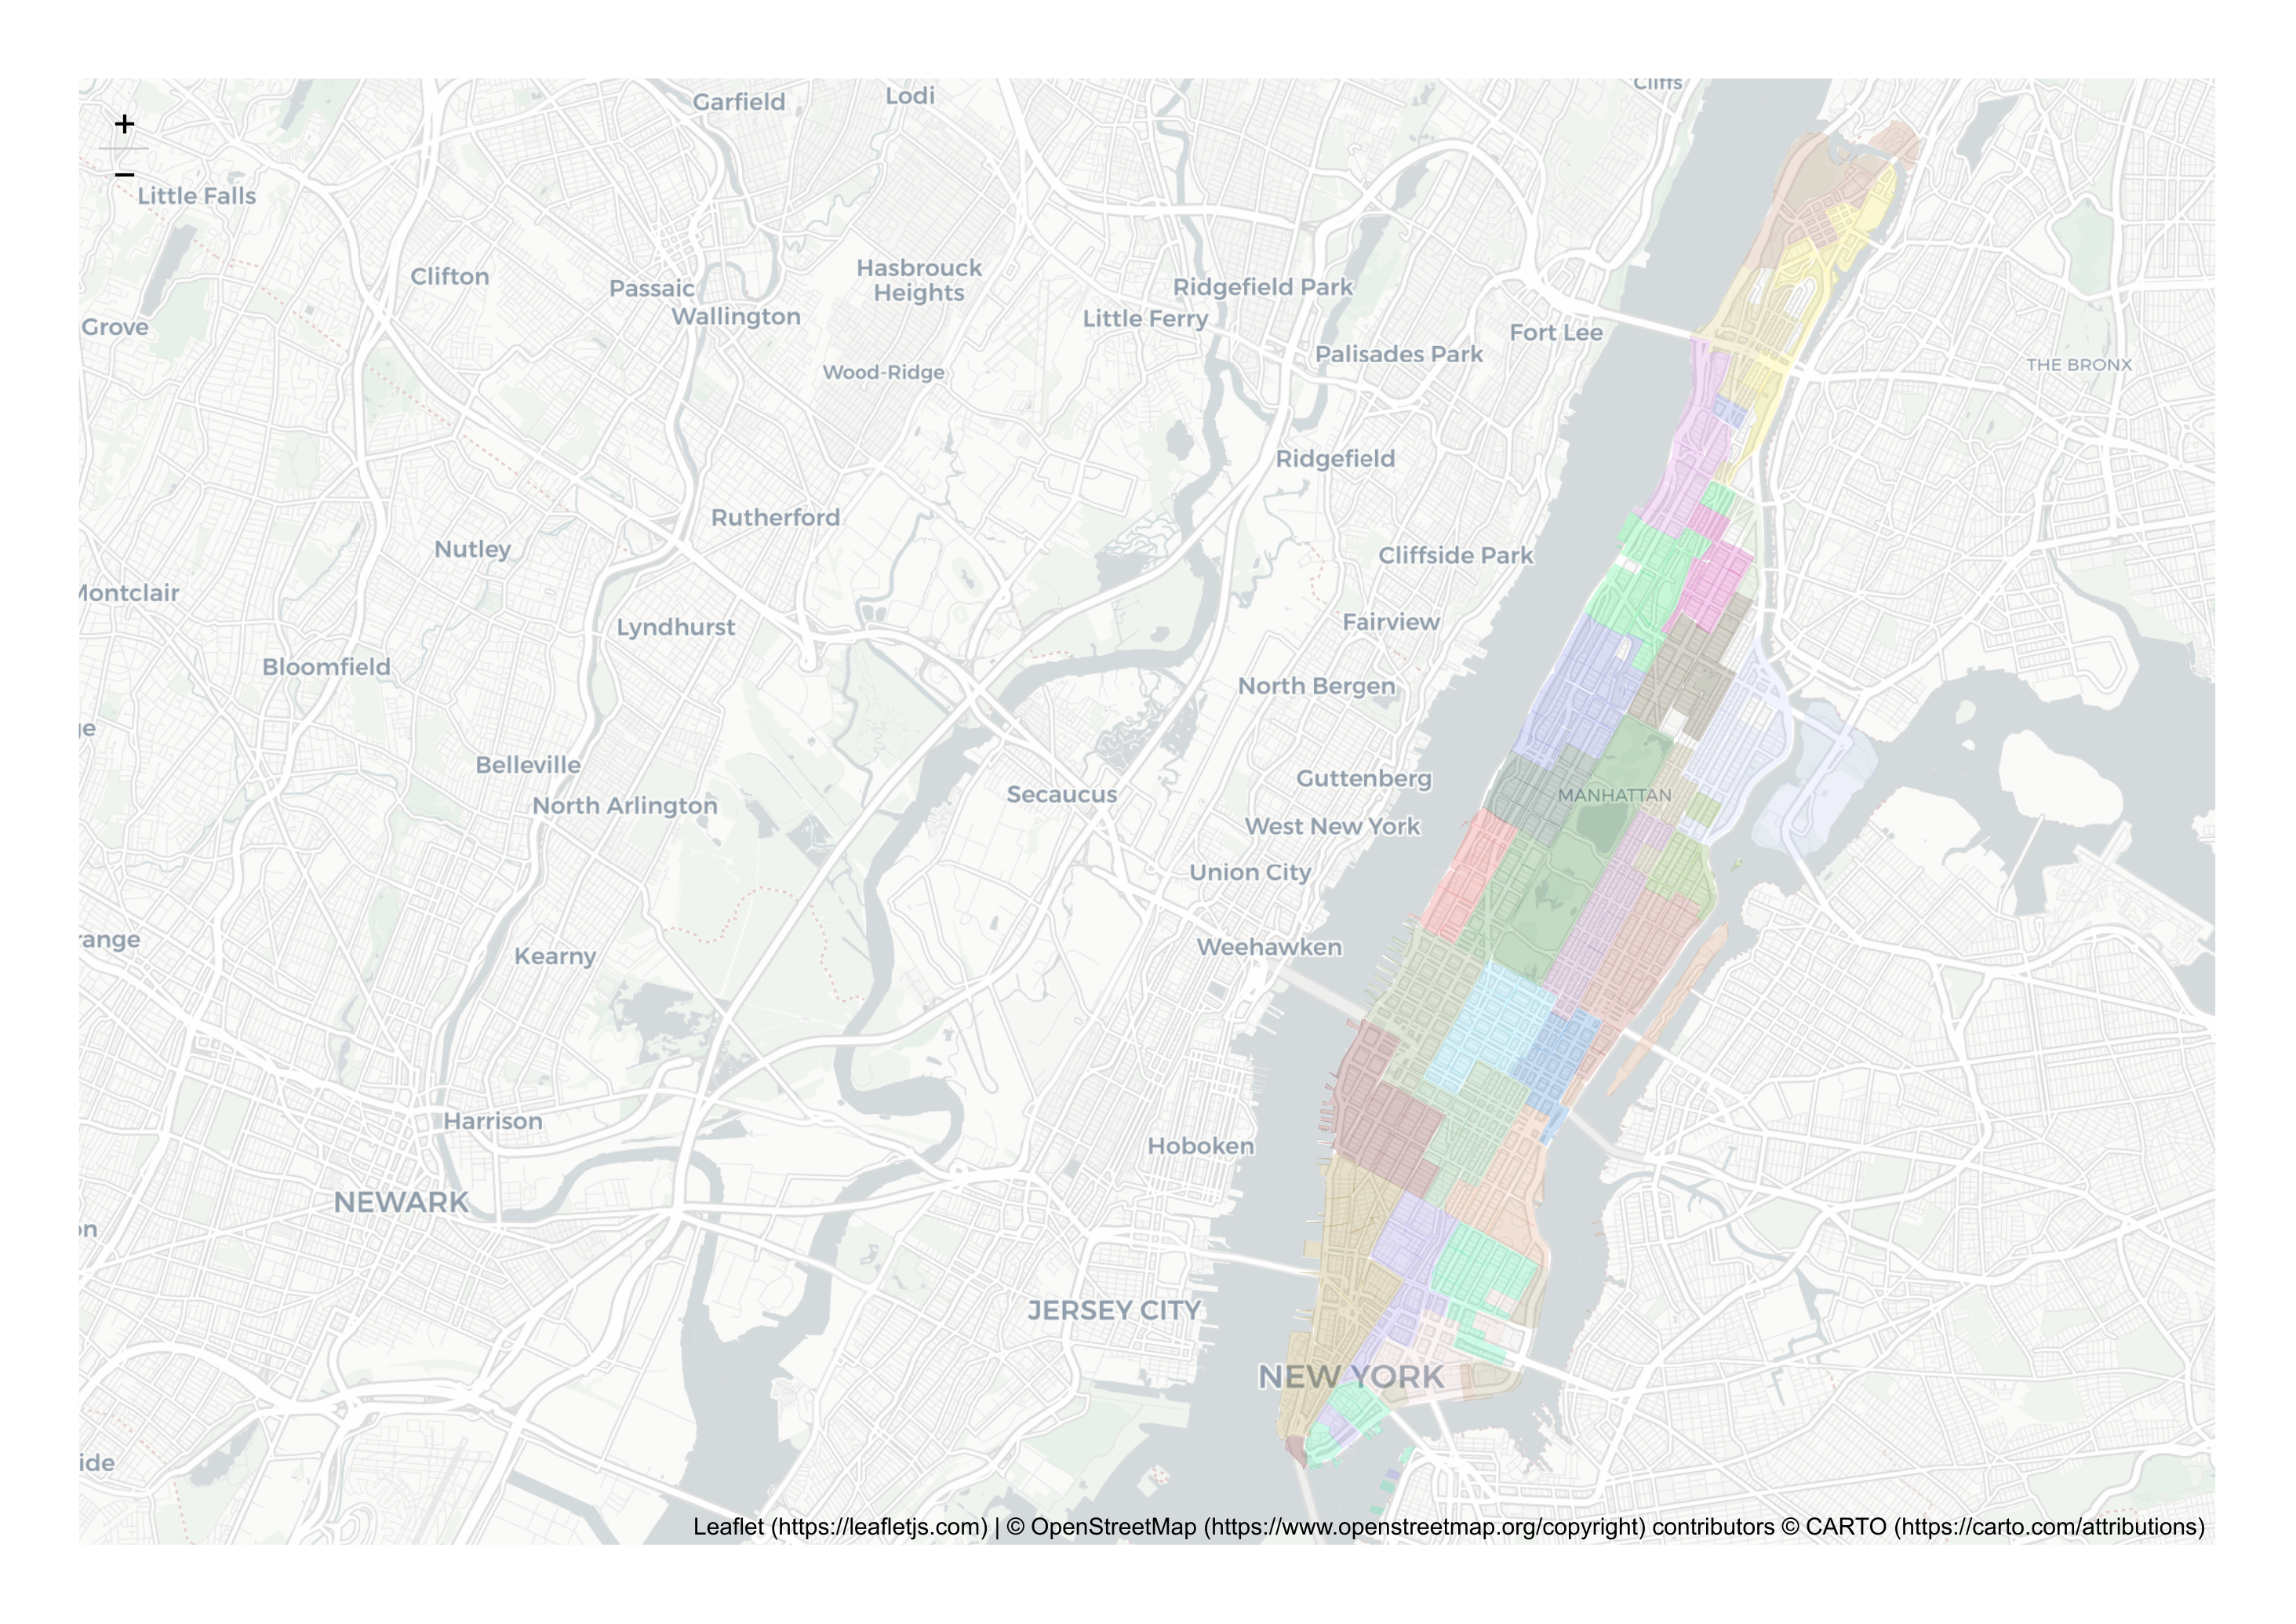}}
		\caption{ReMVC}
		\label{fig:ours}
	\end{subfigure}
	\hspace{0.02\textwidth}
	\begin{subfigure}[b]{0.13\textwidth}
		\fbox{\includegraphics[width=\textwidth]{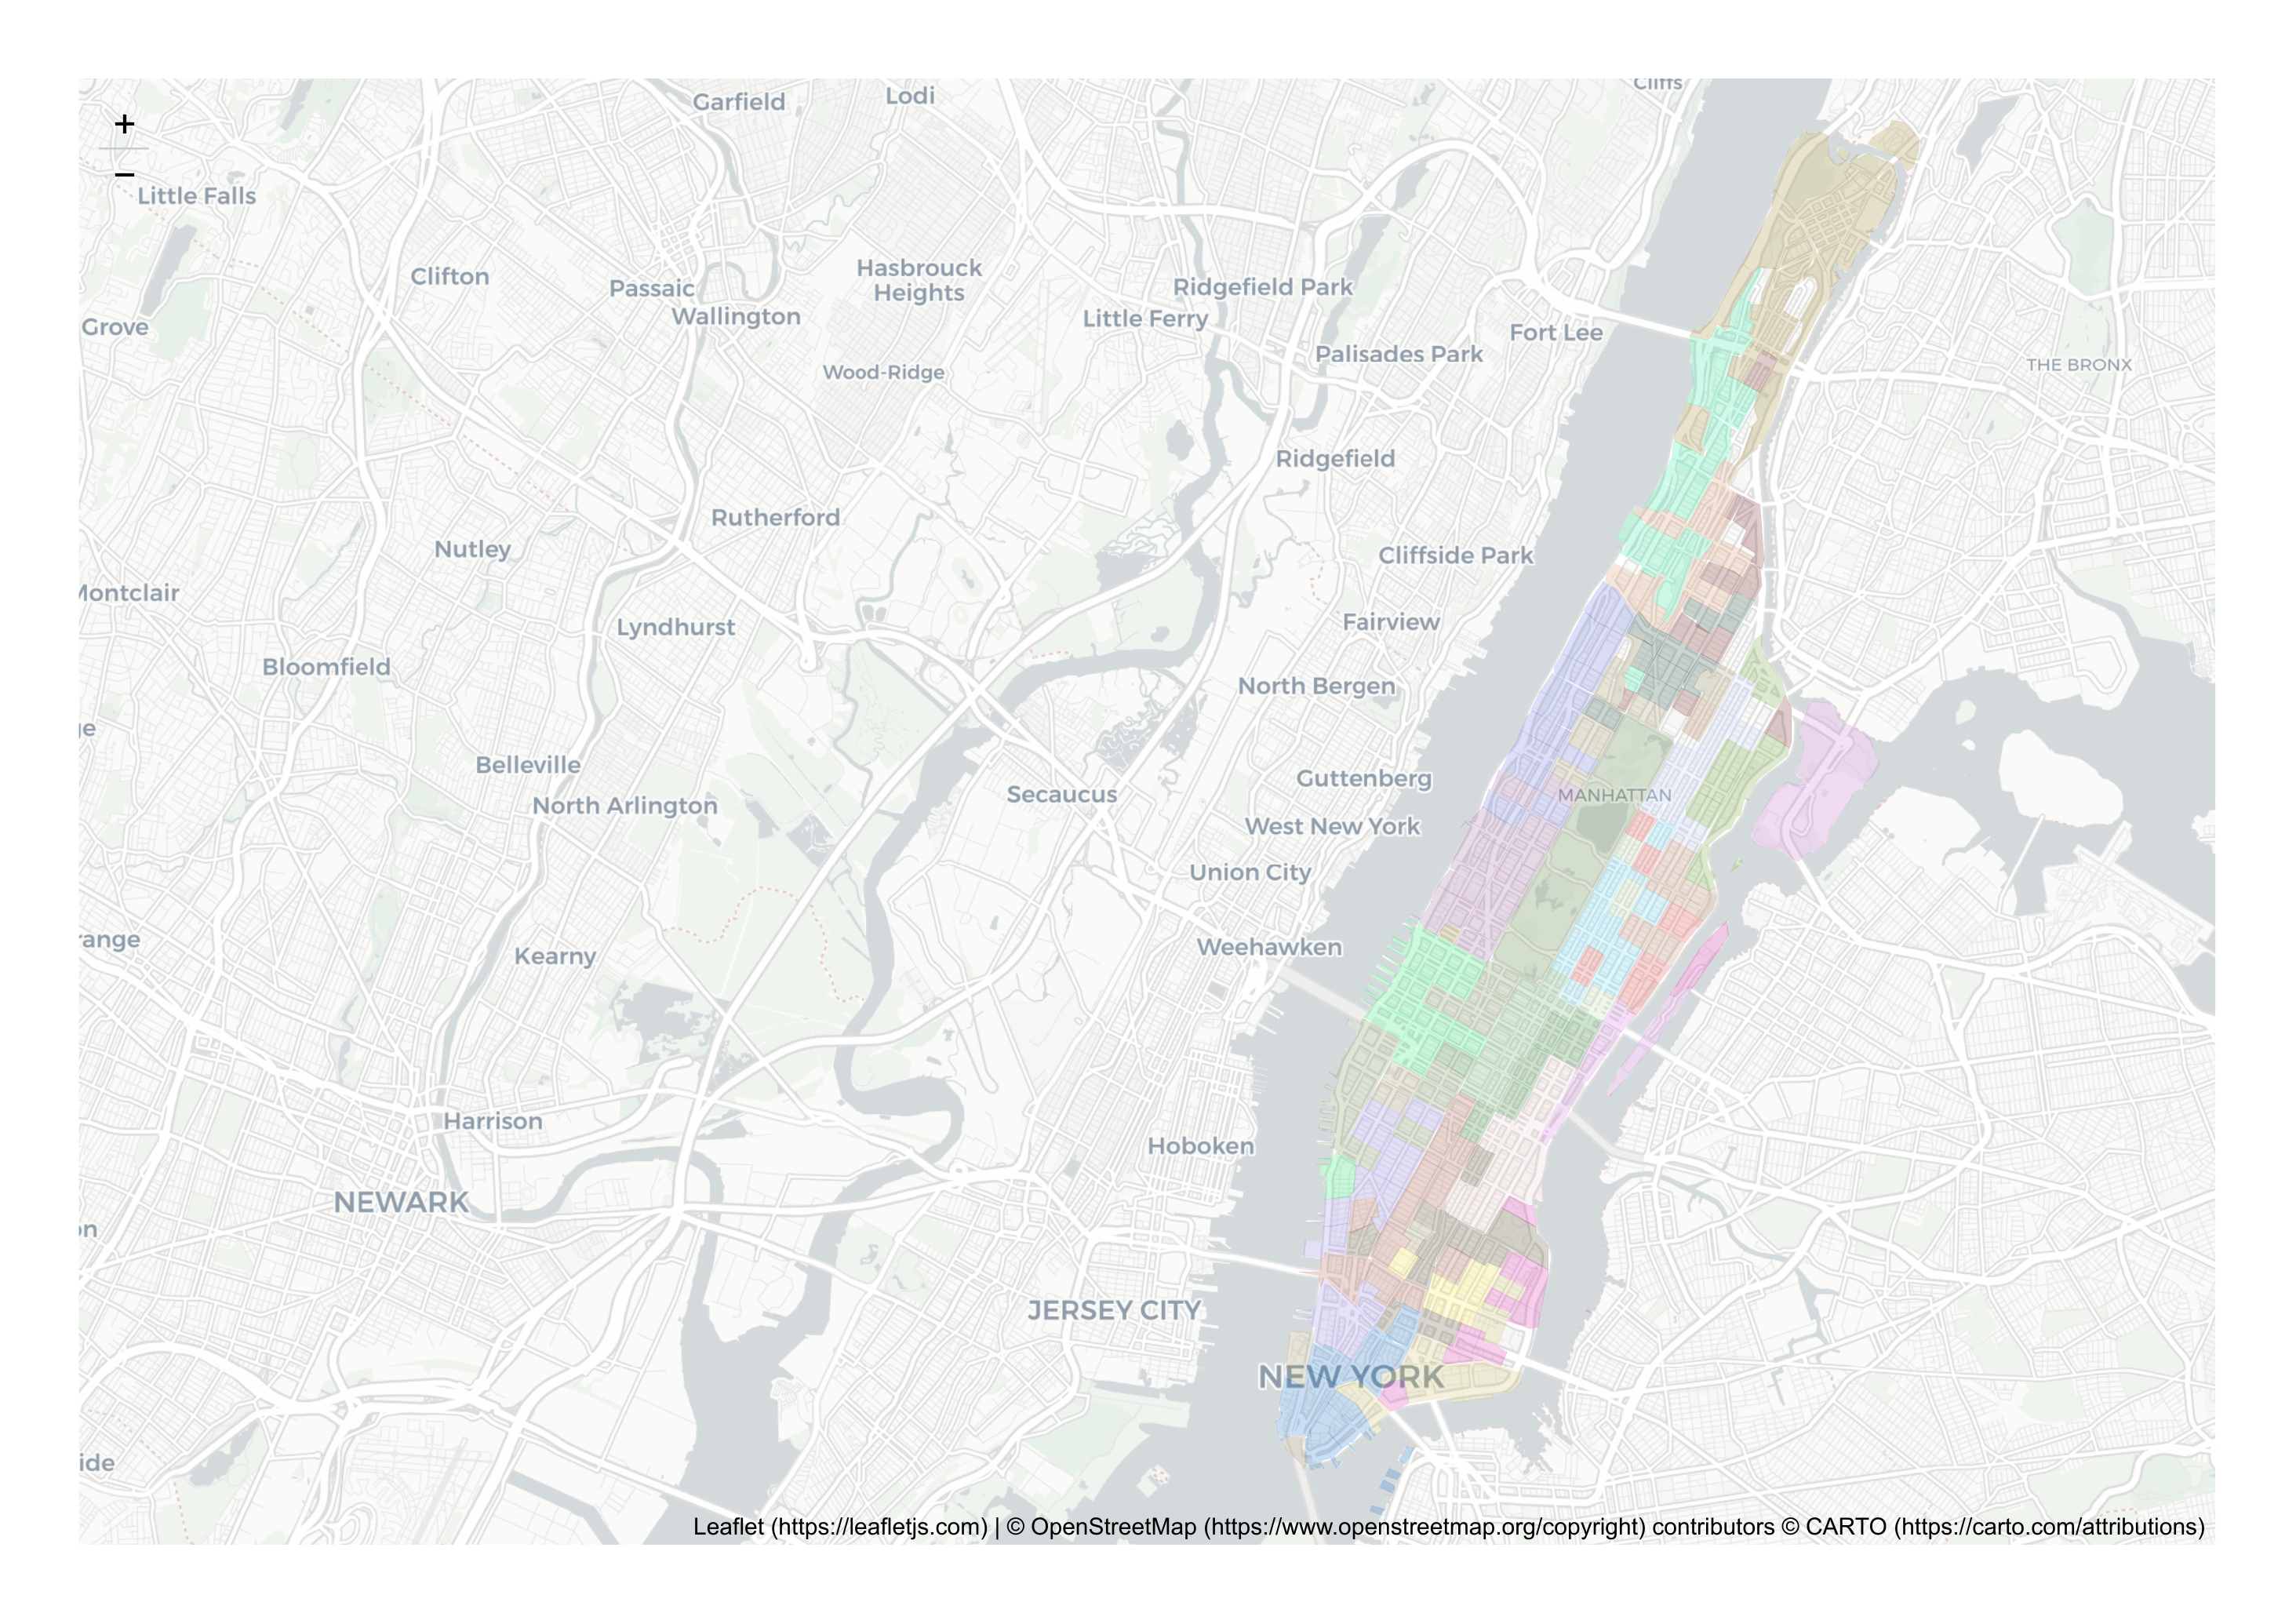}}
		\caption{M2GRL}
		\label{fig:M2GRL}
	\end{subfigure}
	\hspace{0.02\textwidth}
	\begin{subfigure}[b]{0.13\textwidth}
		\fbox{\includegraphics[width=\textwidth]{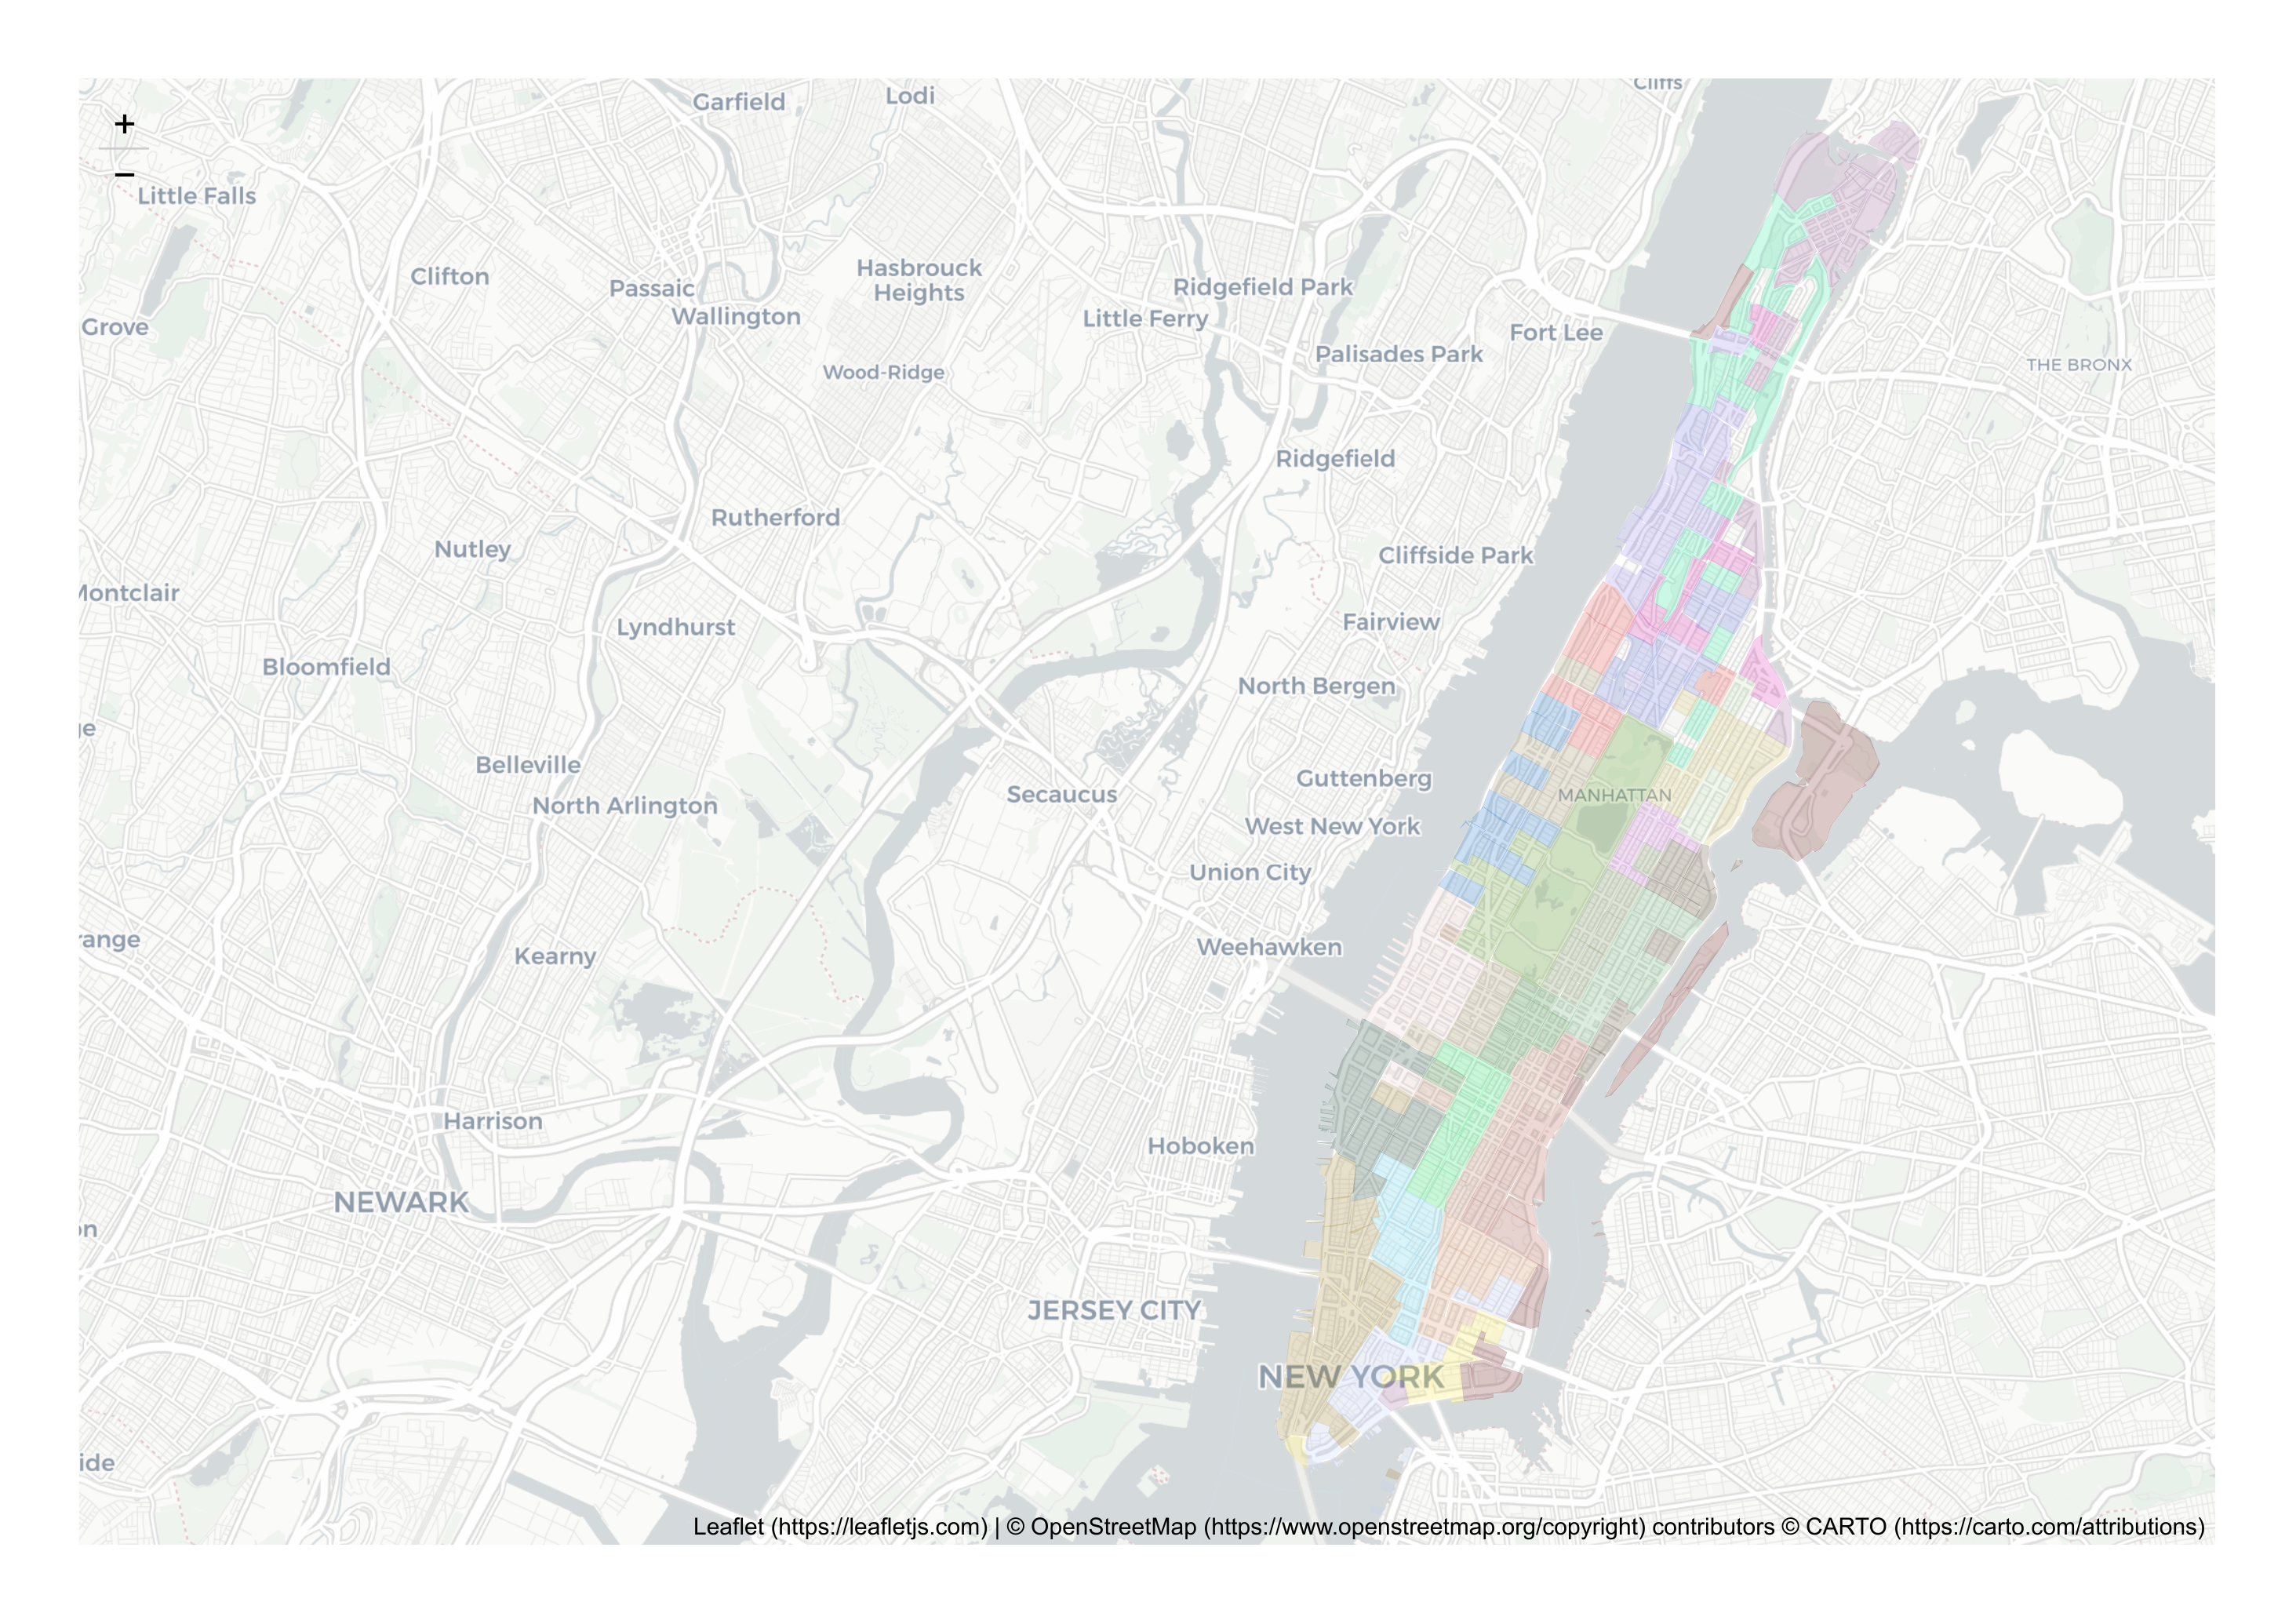}}
		\caption{MVURE}
		\label{fig:MVURE}
	\end{subfigure}
	\hspace{0.02\textwidth}
	\begin{subfigure}[b]{0.13\textwidth}
		\fbox{\includegraphics[width=\textwidth]{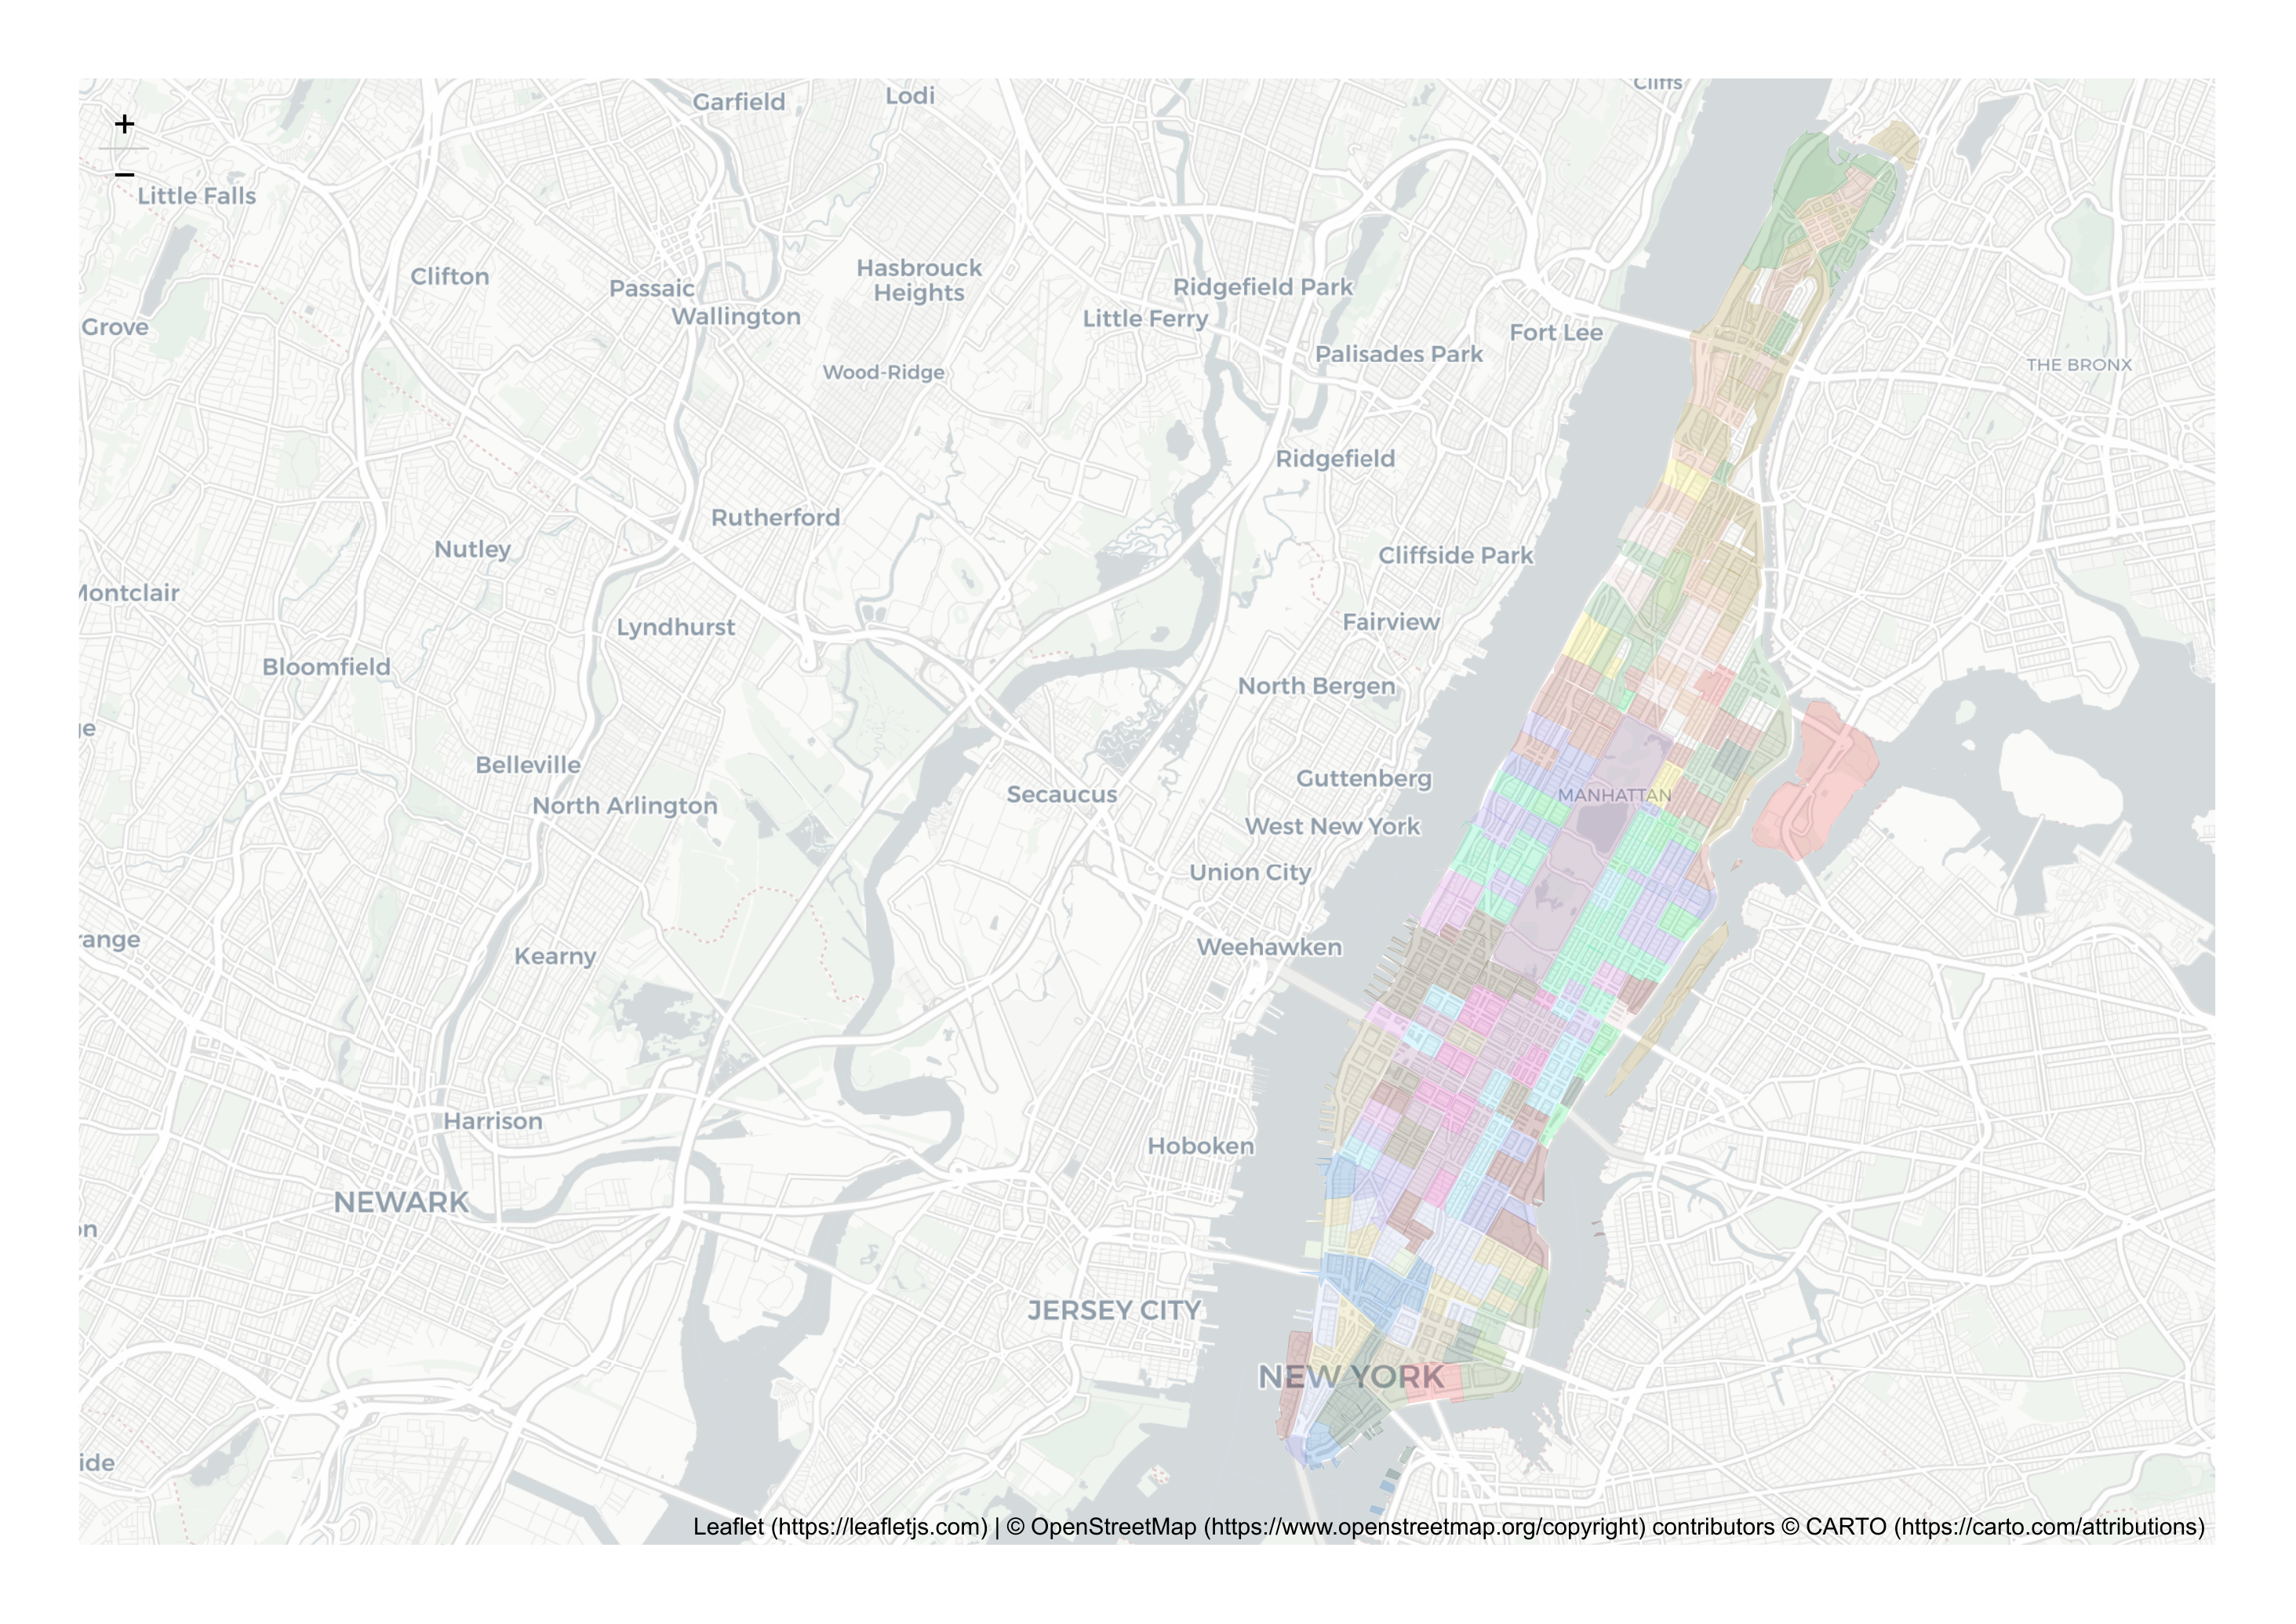}}
		\caption{HDGE}
		\label{fig:HDGE}
	\end{subfigure}
	\hspace{0.02\textwidth}
	\begin{subfigure}[b]{0.13\textwidth}
		\fbox{\includegraphics[width=\textwidth]{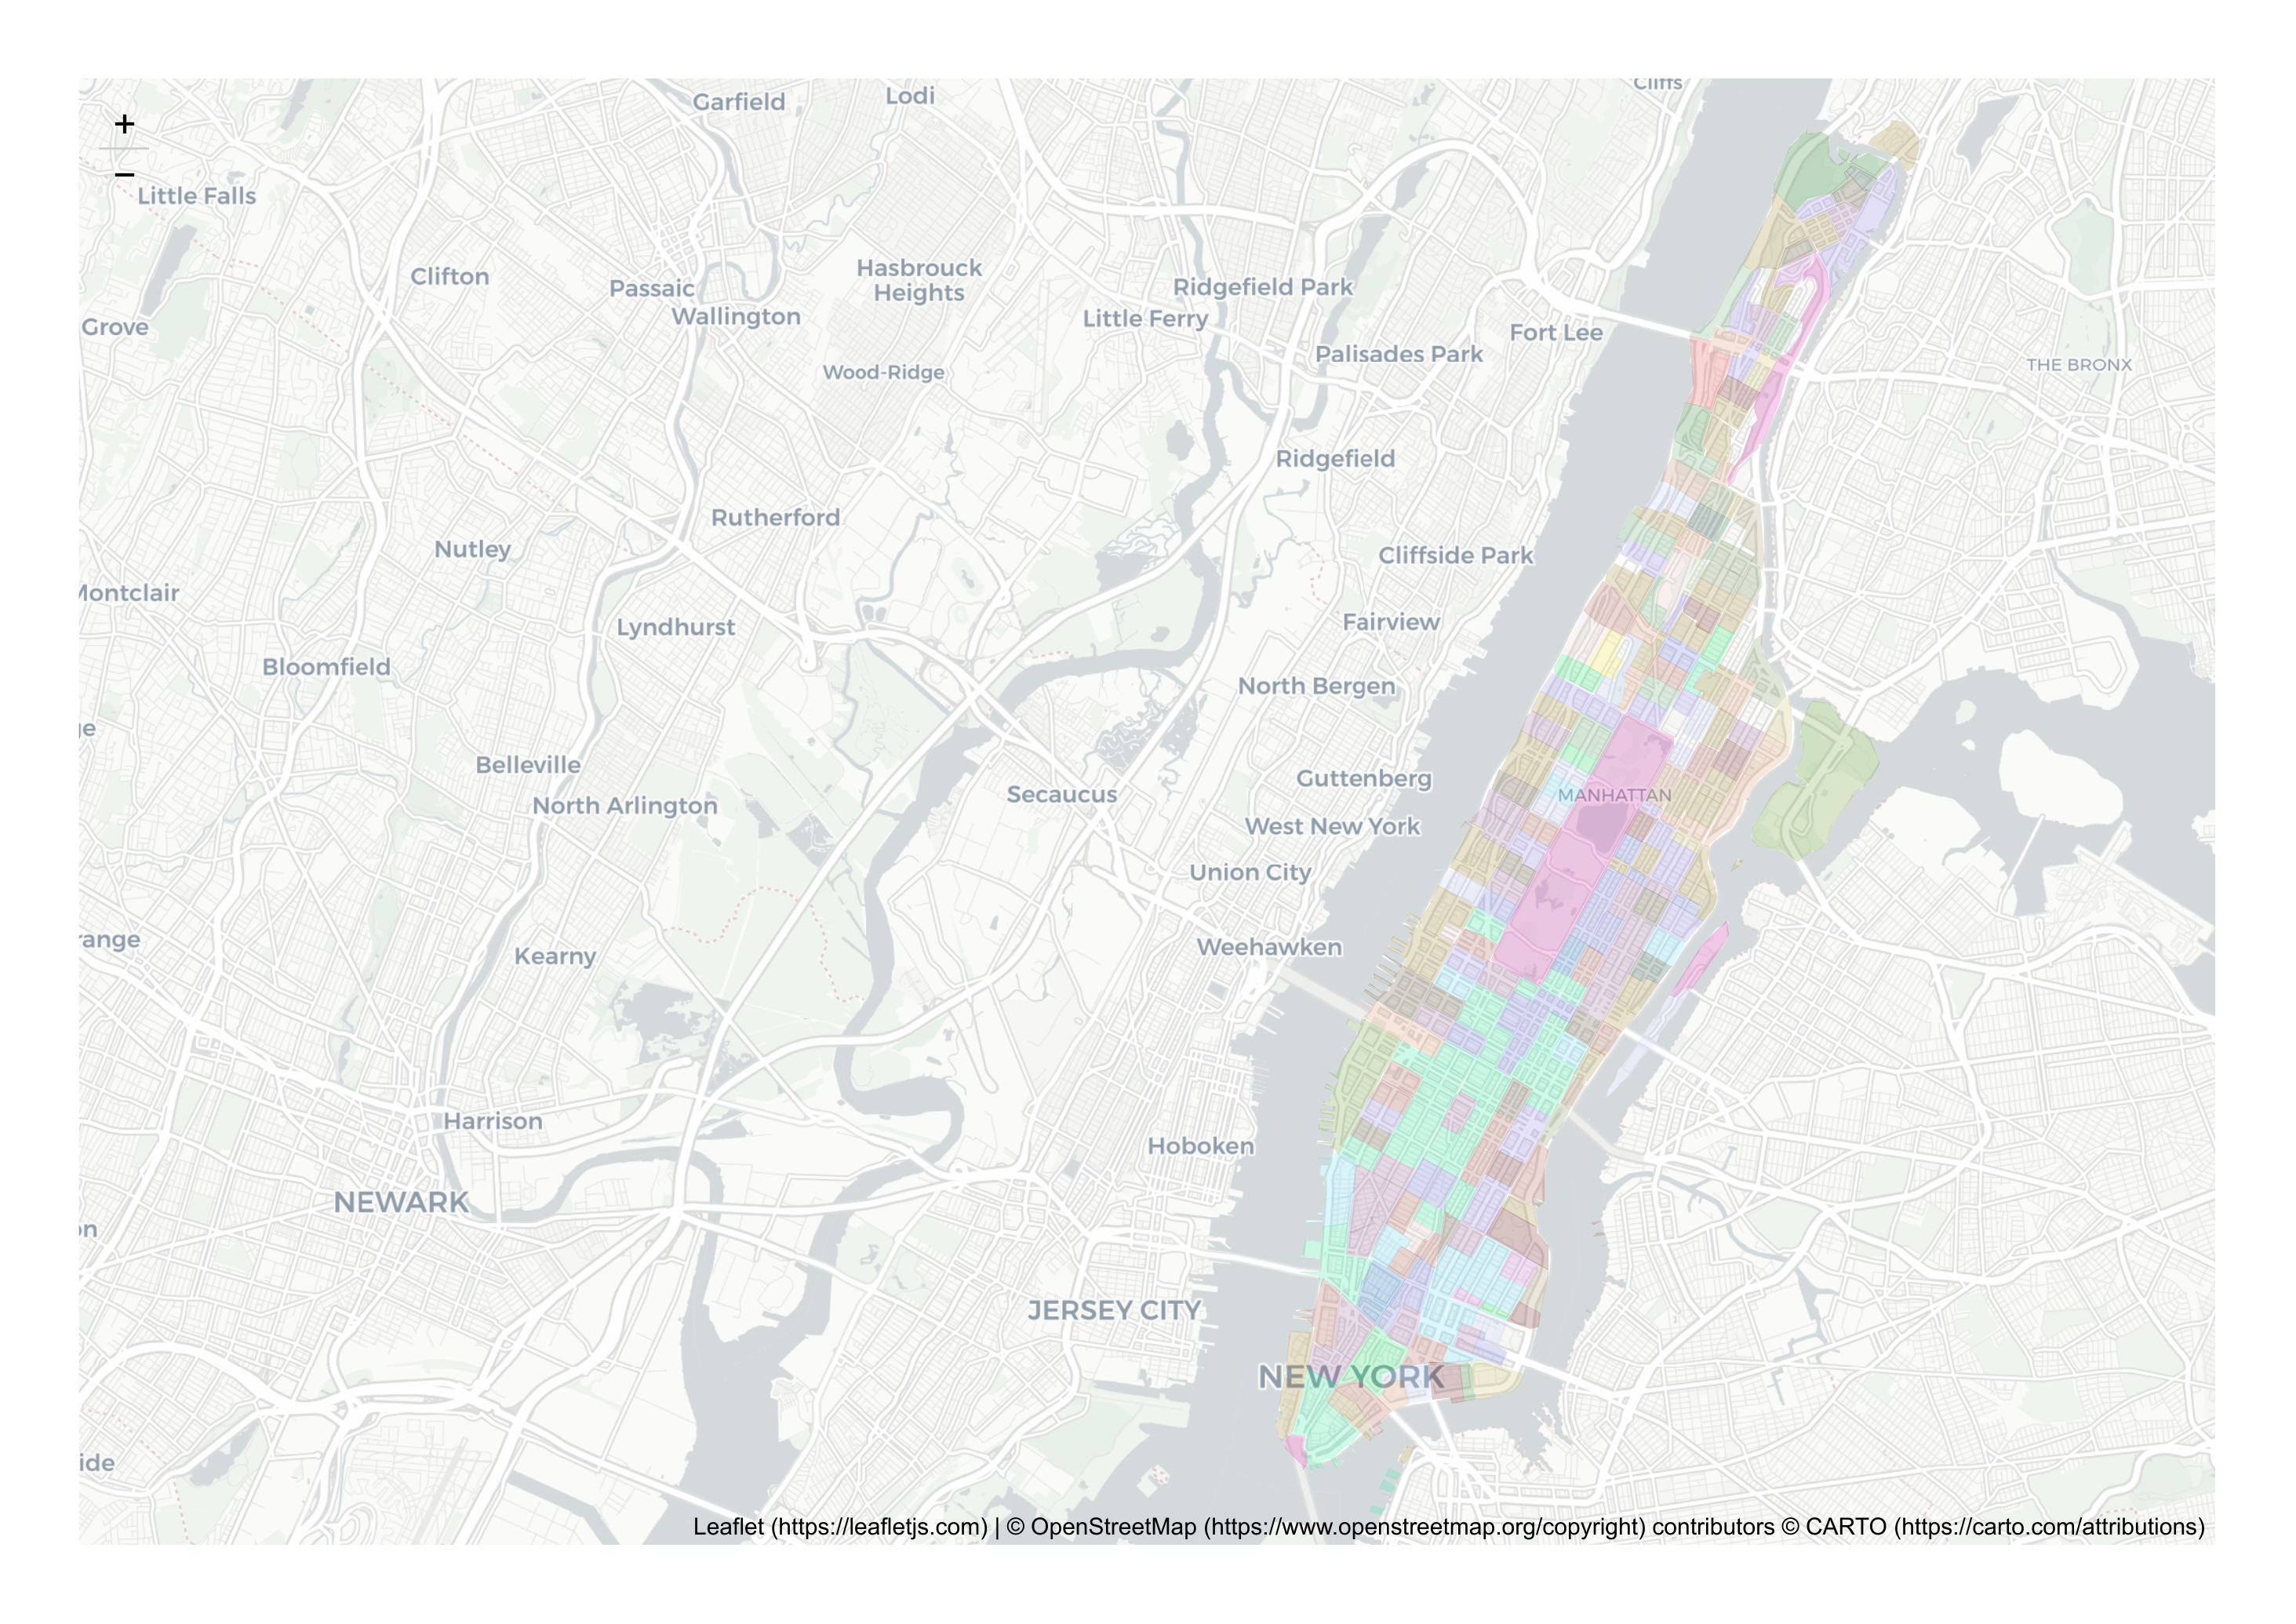}}
		\caption{CGAL}
		\label{fig:CGAL}
	\end{subfigure}
	
	\caption{Districts in Manhattan and region clusters (where the same color means that the regions are in the same cluster).}
	\label{fig:cluster_all}
\end{figure*}

{\FinalOne
\subsection{Comparison with Other Baselines} \label{sec:ccdr}
Another work (CCDR) that uses intra and inter contrastive learning is proposed very recently \citeA{xie2022contrastive_a}. In this paper, each view corresponds user graph data and the intra-view presentation learning is based on graph structure perturbations. However, the urban region graphs do not exist naturally, and pre-defining the region graphs is non-trivial, which may suffer from the drawbacks mentioned in the Introduction section (heuristic-based measures and not learnable). On the other hand, the graph structure perturbations may affect urban function modelling significantly. For example, due to its special POI and flow patterns, the CBD region may only have very sparse connections with other regions. In this case, using structure perturbations (e.g., adding edges or dropping edges) could bring  significant noise and correspondingly the augmented CBD region can not serve as a positive (similar) sample anymore. 
In summary, (1) our method is tailored for region data with POI view and mobility view. It is non-trivial to transform them into suitable graphs. (2) Graph structure perturbations may not be suitable for region-based contrastive learning. (3) CCDR is a supervised method aimed at solving cross-domain recommendation tasks, while our method aims to apply intra- and inter-view contrastive learning for unsupervised region embedding learning for the first time.

% Finally, we compared with CCDR in Table \ref{tab:ccdr_app}. 
{\FinalOne We compare our method and CCDR and show the results in Table~\ref{tab:ccdr_app}.}
For constructing the region graphs, we follow a commonly used strategy named K-nearest neighbor graph (K-NNG). We tune the parameter K among \{10, 20, 30, 40, 50\} and select the best one. From the results, we find that our method performs consistently better than CCDR among two downstream tasks and all metrics. 

\begin{table}[h]
	
	\centering
	\tiny
	\vspace{-0.1cm}
	\caption{Comparision with CCDR (KDD 2022).}
	\vspace{-0.25cm}
	\label{tab:ccdr_app}
	\resizebox{1.0\linewidth}{!}{
		\begin{tabular}{ccccccc}
			\toprule
			\multirow{3}{*}{\textbf{Method}} & \multicolumn{3}{c}{{\it Land Usage Clustering}} & \multicolumn{3}{c}{{\it Popularity Prediction}}  \\
			\cmidrule{2-7}
			& NMI & ARI & F-measure & MAE & RMSE & $R^2$  \\ \midrule
			CCDR & 0.655 & 0.268 & 0.294 & 248.31 & 379.40 & 0.414 \\
			ReMVC & \textbf{0.762} & \textbf{0.474} & \textbf{0.488} & \textbf{189.92} & \textbf{296.26} & \textbf{0.643} \\
	\bottomrule
	\end{tabular}}
	\vspace{-0.2cm}
\end{table}
}

\subsection{Complete Visualization For Land Use Clustering} 
Fig. \ref{fig:cluster_all} shows the complete clustering results of five methods that have the top ARI scores, namely ReMVC, M2GRL, MVURE, HDGE and CGAL.
% We also visualize the clustering results of five methods that have the top ARI scores, namely ReMVC, M2GRL, MVURE, HDGE and CGAL, in Fig. \ref{fig:cluster}, 
where the same color means that the regions are in the same cluster. For HDGE, the functional regions are weakly identified since only human mobility data is used. %The POI categories play an important role in region cluster identification. For example, with more parks and bars, a region is more likely to be an entertainment region. 
CAGL cannot identify the correct region cluster either since it cannot effectively fuse multi-view information but mainly depends on POI modeling. M2GRL and MVURE provides better performance than other baselines and obtains more reasonable clusters. However, some clusters are still mixed with each other especially on the middle part. In contrast, ReMVC gives the most satisfying identification with clear cluster boundaries, which demonstrates that the region functionalities are well preserved by our model. 

\subsection{Ablation Study for Other Modules} \label{sec:as}
In this experiment, we further inspect how other modules (besides contrastive learning and multi-view cooperation which have been studied in Section \ref{ablation}) of ReMVC affect the model performance. 

% To investigate the impacts of negative sampling methods, we replace the feature distance based sampling with random sampling in model ReMVC-RS. We also replace the feature extractor of $G^p$ and $G^m$ with another commonly used structure CNN with the kernel size of 7 and rename this model as ReMVC-CNN. As for the embedding fusion operations, we consider these commonly used fusion operations, including Average, Max, Gated, Neural Networks (NN) based and Bilinear fusion, for comparison.

{\FinalOne
To further investigate the necessity of % hierarchica 
intra and inter-view contrastive learning from another perspective, we propose a cross view augmentation strategy to facilitate knowledge propagation directly in the base model ReMVC-CA instead of using the high-level inter-view contrastive learning. Specifically, taking the mobility view as an example. When {\FinalOne constructing} the positive region set for the $k$-th region $r_k$, in addition to intra-view augmentation $\mathcal{A}_m$, we define cross-view augmentation as the top-$K$ ($K=3$) regions, {\FinalOne which are the most} similar to $r_k$ in the POI view (vice versa). 

We also study the design of inter-view contrastive learning by replacing the ``correlations'' based one-to-one mapping classification task in Equation \ref{eq:inter} with a similarity constraint-based task implemented as inner product. We call the new variant the ReMVC-Sim model. 

To investigate the impacts of negative sampling methods, we replace the feature distance based sampling with Euclidean distance based sampling in model ReMVC-ES and random sampling in model ReMVC-RS respectively, where Euclidean distance based sampling means that the sampling probability for a candidate region $r_n$ is defined as the normalization of its physical distance from the anchor region $r_k$ and the random sampling means that the sampling probability is uniform.} 

We also replace the feature extractor of $G^p$ and $G^m$ with another commonly used structure CNN with the kernel size of 7 and rename this model as ReMVC-CNN. As for the embedding fusion operations, we consider these commonly used fusion operations, including Average, Max, Gated, Neural Networks (NN) based and Bilinear fusion, for comparison.

From experiment results in Table \ref{tab:fusion}, we can have the following observations: {\FinalOne (1) We can find that ReMVC brings huge improvement compared with ReMVC-CA, showing that our model does benefit from the hierarchical structural design of contrastive learning. This result is consistent with the finding indicated by comparing ReMVC with w/o IV in Section \ref{ablation}. (2) As for inter-view task design, we can find that our method ReMVC outperforms ReMVC-Sim {\FinalOne by} about 45\% in F-measure and 28\% in $R^2$. The underlying reason is that preserving similarity between views instead of correlation brings noise and leads to the same multi-view representations, which is detrimental to downstream tasks. (3) As for different sampling methods, we can find that ReMVC outperforms ReMVC-ES on two downstream tasks consistently, showing that the Euclidean distance sampling can hardly define effective negative regions. The possible reason is that regions far away on the map may still serve as similar urban functions. In addition, it is also  unreasonable to treat regions with various functions equally. Thus, ReMVC outperforms ReMVC-RS for about 8\% in land usage clustering task and  17\% in popularity prediction task.} 
(4) ReMVC achieves better results than ReMVC-CNN on both clustering and regression tasks, showing the superior ability of MLP for intra-view feature extraction. (5) Among the studied fusion operations, the max fusion performs better in the land usage clustering task while the NN based fusion performs better in the popularity prediction task. However, all these operations lead to entangled region representations. Instead, the disentangled multi-view representation by concatenation (adopted in this paper) can achieve the best results and the inter-view contrastive learning serves to propagate information across views. 

\begin{table}[h]
	
	\centering
	\tiny
	%\vspace{-0.25cm}
% 	\vspace{-0.1cm}
	\caption{Ablation Study for Other Modules.}
% 	\vspace{-0.25cm}
	\label{tab:fusion}
	\resizebox{1.0\linewidth}{!}{
		\begin{tabular}{c|ccc|ccc}
			\toprule
			\multirow{2}{*}{\textbf{Method}} & \multicolumn{3}{c|}{{\it Land Usage Clustering}} & \multicolumn{3}{c}{{\it Popularity Prediction}}  \\
			\cmidrule{2-7}
			& NMI & ARI & F-measure & MAE & RMSE & $R^2$  \\ \midrule
			ReMVC-CA & 0.753 & 0.443 & 0.451 & 251.91 & 376.45 & 0.420 \\
			ReMVC-Sim & 0.668 & 0.303 & 0.327 & 229.65 & 348.83 & 0.502 \\ \midrule
			ReMVC-ES & 0.751 & 0.442 & 0.457 & 255.81 & 387.65 & 0.385
			\\ 
			ReMVC-RS & 0.751 & 0.436 & 0.452 & 228.32 & 363.75 & 0.459 \\ \midrule
			ReMVC-CNN & 0.742 & 0.434 & 0.464 & \underline{202.59} & \underline{315.71} & \underline{0.595} \\ \midrule
			Average & 0.756 & 0.449 & 0.458 & 231.02 & 353.47 & 0.489  \\
			Max & \underline{0.759} & \underline{0.466} & \underline{0.471} & 238.06 & 365.77 & 0.455  \\
			Gated & 0.736 & 0.414 & 0.432 & 246.38 & 380.54 & 0.408 \\
		    NN Based & 0.560 & 0.154 & 0.182 & 236.12 & 347.02 & 0.508 \\
			Biliner & 0.721 & 0.388 & 0.407 & 231.83 & 360.54 & 0.468 \\
			\cmidrule{1-7}
			ReMVC & \textbf{0.762} & \textbf{0.474} & \textbf{0.488} & \textbf{189.92} & \textbf{296.26} & \textbf{0.643} \\ \bottomrule
	\end{tabular}}
% 	\vspace{-0.4cm}
\end{table}

\begin{figure}[t!]
	\centering
	\begin{subfigure}[b]{0.45\textwidth}
		\includegraphics[width=\textwidth]{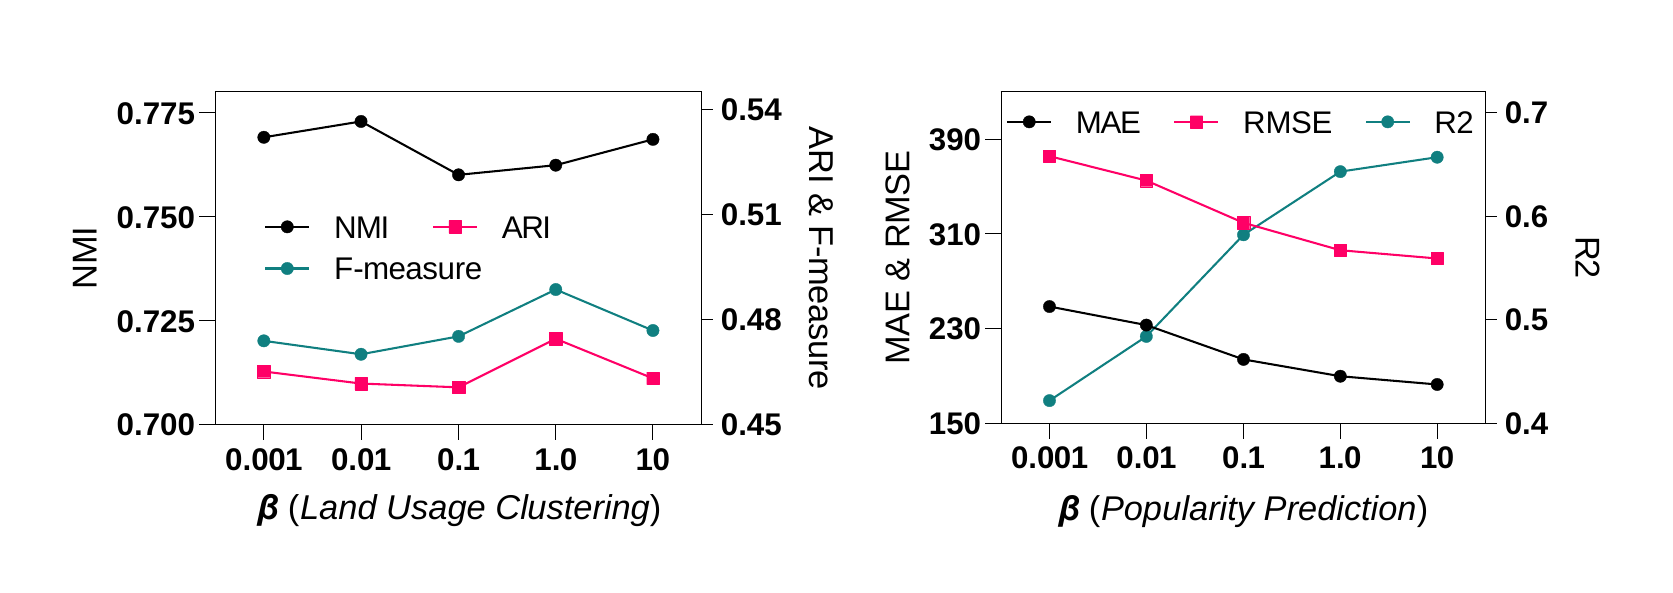}
		\caption{Parameter $\beta$}
		\label{fig:beta}
	\end{subfigure}
	\vspace{-0.2cm}
	\begin{subfigure}[b]{0.45\textwidth}
		\includegraphics[width=\textwidth]{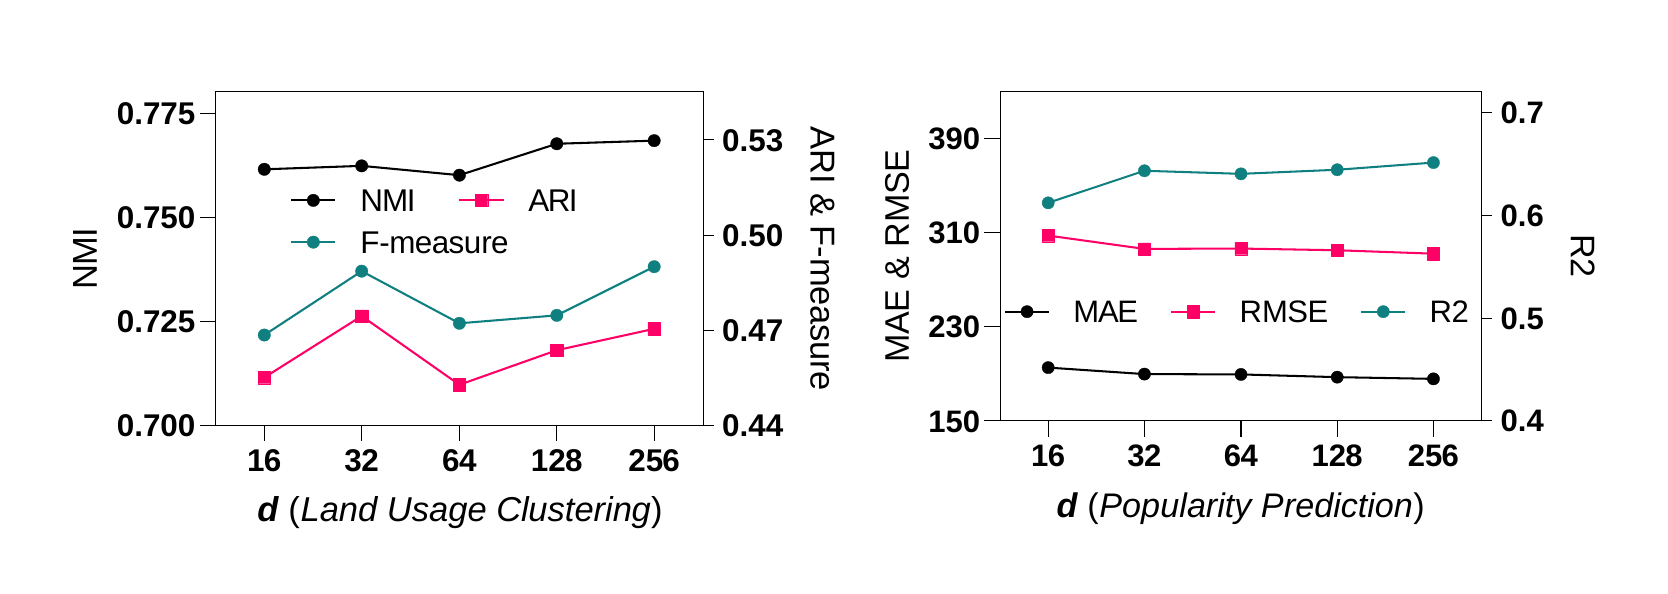}
		\caption{Parameter $d$}
		\label{fig:d}
	\end{subfigure}
	\caption{Impact of hyper-parameters $\beta$ and $d$.}
    \vspace{-0.3cm}
	\label{fig:sense_all}
\end{figure}

\begin{figure}[ht]
	\centering
	\begin{subfigure}[b]{0.45\textwidth}
		\includegraphics[width=\textwidth]{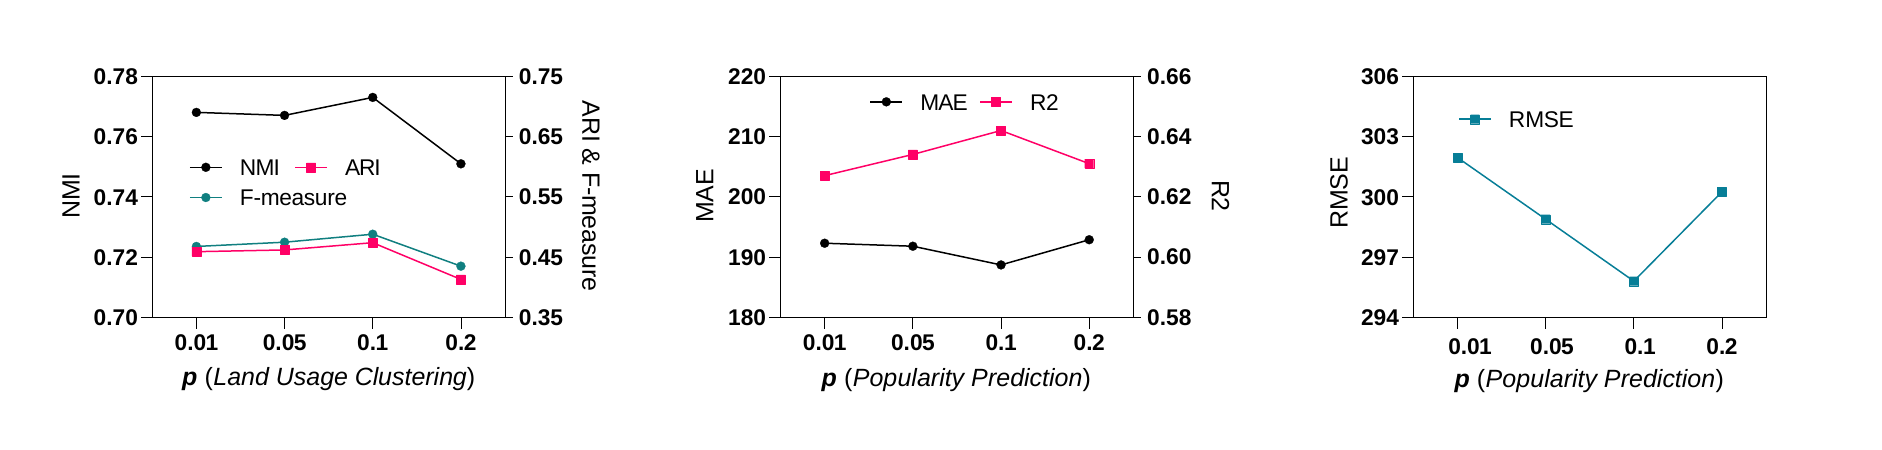}
		\caption{Parameter $p$}
		\label{fig:p}
	\end{subfigure}
	\vspace{-0.2cm}
	\begin{subfigure}[b]{0.45\textwidth}
		\includegraphics[width=\textwidth]{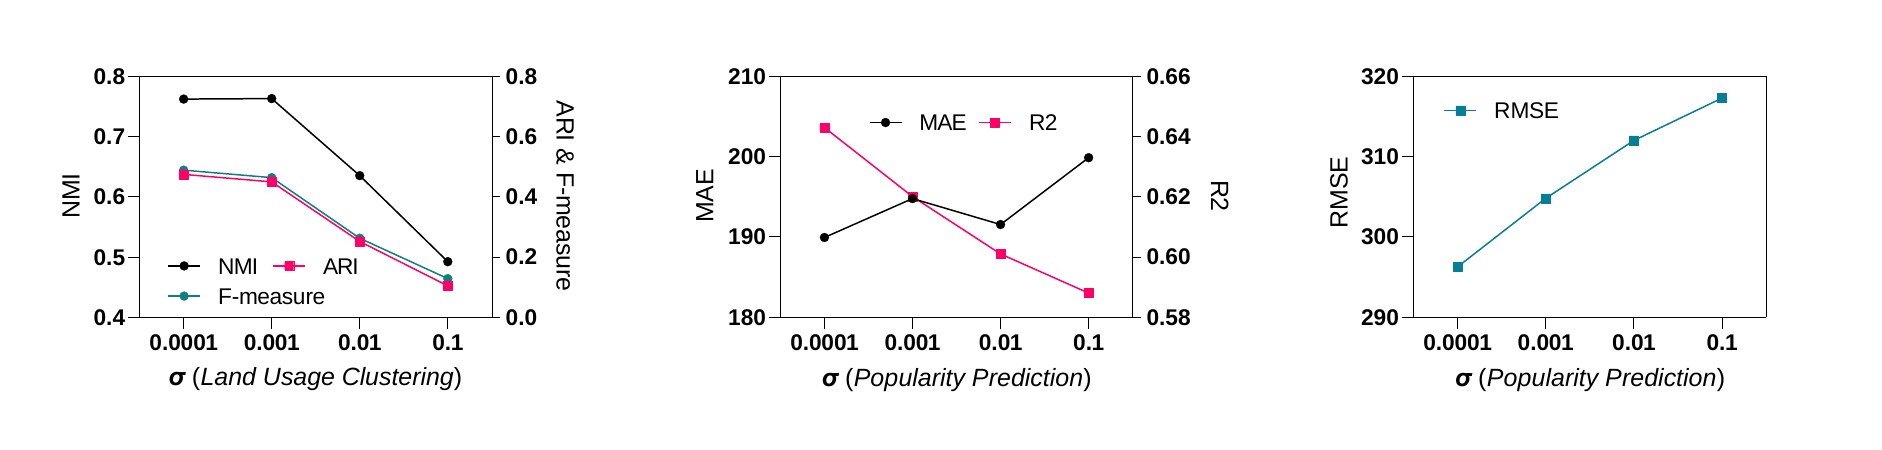}
		\caption{Parameter $\sigma$}
		\label{fig:sigma}
	\end{subfigure}
	\caption{Impact of hyper-parameters $p$ and $\sigma$.}
	\label{fig:sense_all}
\end{figure}

\subsection{Parameter Analysis} \label{sec:app_pa}
% We conduct the parameter study on the weighted parameter $\beta$, $\alpha$ in Eq. \ref{eq:loss}, the embedding size $d$, and the parameters $p$ and $\sigma$ for defining the augmentation operations for POI view and mobility view, respectively. 

{\FinalOne
We conduct the parameter study on the weighted parameter $\beta$, $\alpha$ in Eq. \ref{eq:loss}, the embedding size $d$, the parameters $p$ and $\sigma$ for defining the augmentation operations for POI view and mobility view, and negative sizes $N_p$, $N_m$, $N_i$ for intra/inter views respectively. 
}

%Due to the page limit, we present the results on the first three here and put those on others in the supplementary materials.

%{\ChengComment We conduct the parameter study on the weighted parameter $\beta$, $\alpha$ in Eq. \ref{eq:loss}, the embedding size $d$, and the parameters $p$ and $\sigma$ for defining the augmentation operations for POI view and mobility view, respectively. Due to the page limit, we present the results on the first three here and put those on others in the supplementary materials.}

\textbf{The weighted parameter $\beta$ and $\alpha$.} As can be seen in Fig.~\ref{fig:beta}, the model performance would fluctuate with different values of $\beta$. 
%For the land usage clustering task, 0.01 is the best setting for NMI while 1.0 is the best for other metrics. The results are reasonable because both ARI and F-measure regard the clustering results as a series of binary classification decisions. 
While ReMVC remains relatively stable on clustering task, it %seems to be 
is more sensitive to this parameter in popularity prediction. 
%The model performance increases with $\beta$ and then begins to be stable when $\beta$ is larger than 1.0. 
The performances when $\beta=0.001$ cannot compete with that when $\beta$ gets larger, which conforms to the results in ablation study and again show the necessity of introducing the inter-view contrastive learning module for cross-view information sharing. We omit the discussion for $\alpha$ because it obtains the similar results. 

\textbf{Embedding size $d$.} Fig.~\ref{fig:d} shows the impact of embedding size on the results. The model is quite robust under different embedding sizes ranging from 16 to 256, with the largest difference being less than 2\%. It is also interesting to discover that using high-dimensional representation does not always produce the best results. For example, ARI and F-measure achieve the best when $d=32$. %The robustness against embedding size is useful in real scenarios since it can significantly reduce memory usage.

% In this section, we show the experiment results for the other two important parameters, \textit{i.e.}, augmentation probability $p$ and Gaussian variance $\sigma$. 

\textbf{The augmentation probability $p$ for POI view.} As can be seen in Fig.~\ref{fig:p}, the model performance would fluctuate with different values of $p$, where 0.1 is the best setting for both tasks. The results are reasonable because each region only includes a small amount of POIs. Meaningful augmentations are hard to generate with a small $p$. In fact, the augmentation is likely to be the anchor region itself so that the model cannot obtain informative positive samples. %In contrast
On the other hand, when $p$ is too large, the augmentations introduce much noise and may affect the model learning. 

\textbf{The Gaussian variance $\sigma$ for Mobility view.} Fig.~\ref{fig:sigma} shows the impact of various Gaussian variances on the results. We can find that the model performance decreases with $\sigma$ for both tasks. The possible reason is that the injected noise with large $\sigma$ will dominate the true origin/destination distributions and hence the model accepts questionable positive samples.

\begin{figure}[ht]
	\centering
	\begin{subfigure}[b]{0.45\textwidth}
		\includegraphics[width=\textwidth]{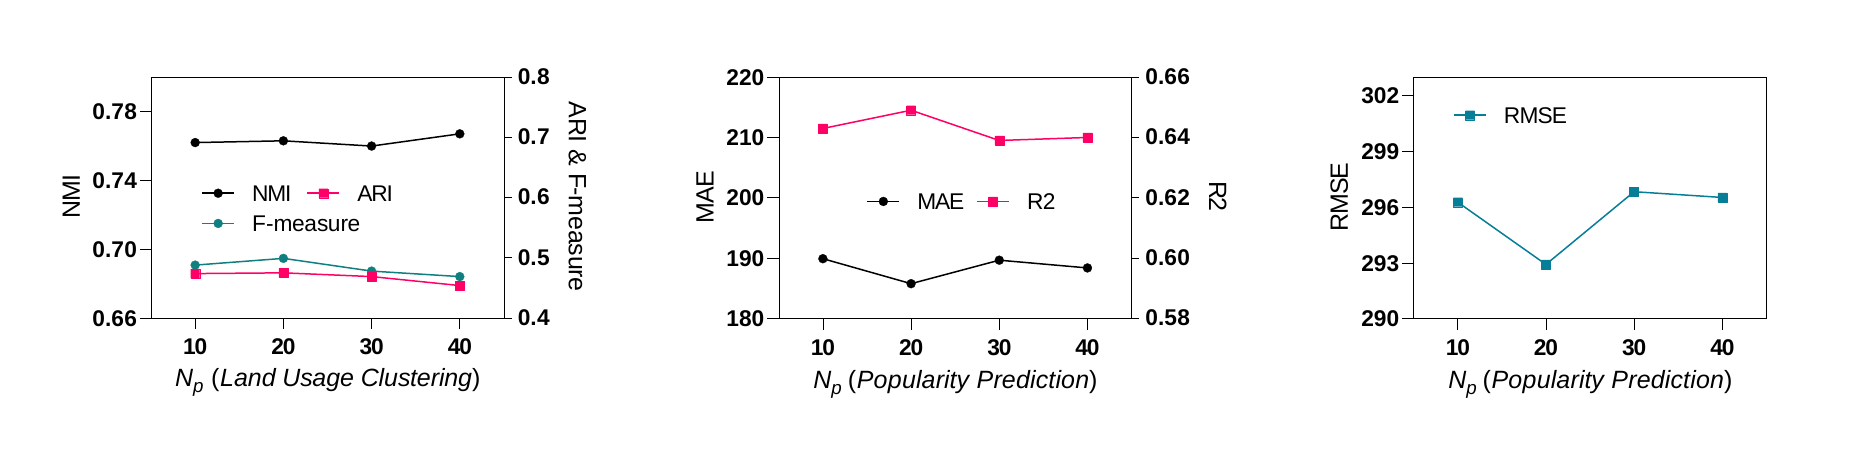}
		\caption{Parameter $N_p$}
		\label{fig:np}
	\end{subfigure}

	\begin{subfigure}[b]{0.45\textwidth}
		\includegraphics[width=\textwidth]{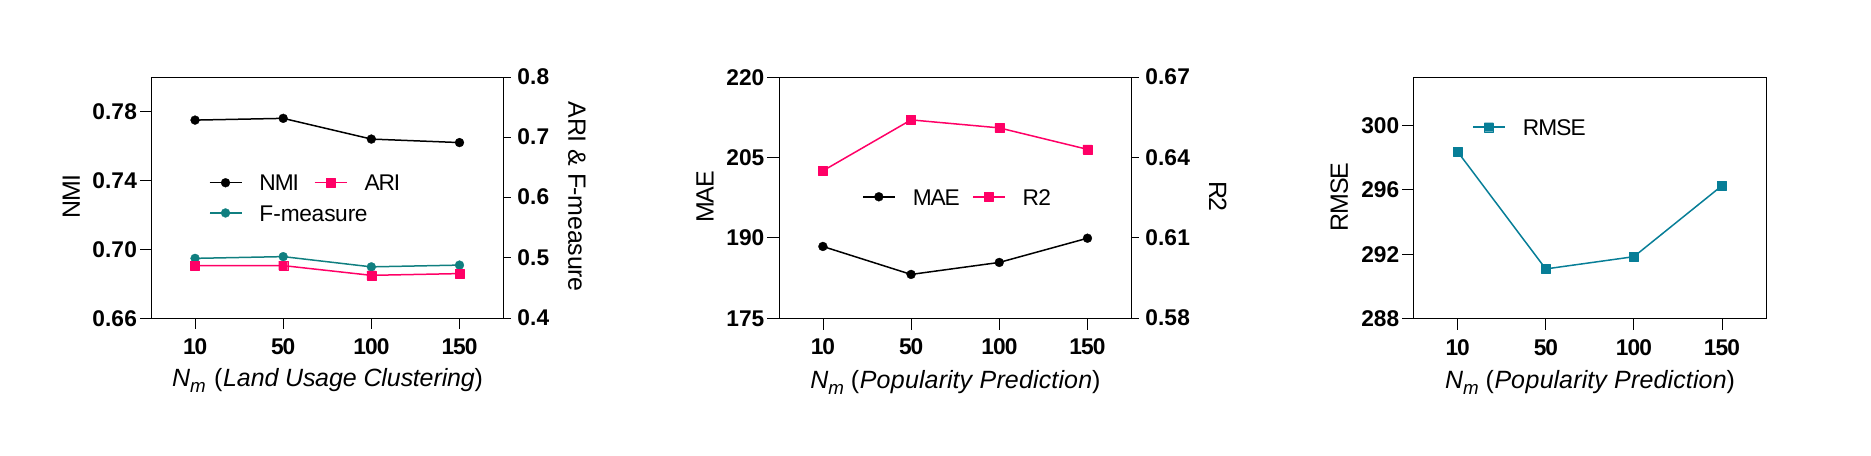}
		\caption{Parameter $N_m$}
		\label{fig:nm}
	\end{subfigure}

	\begin{subfigure}[b]{0.45\textwidth}
		\includegraphics[width=\textwidth]{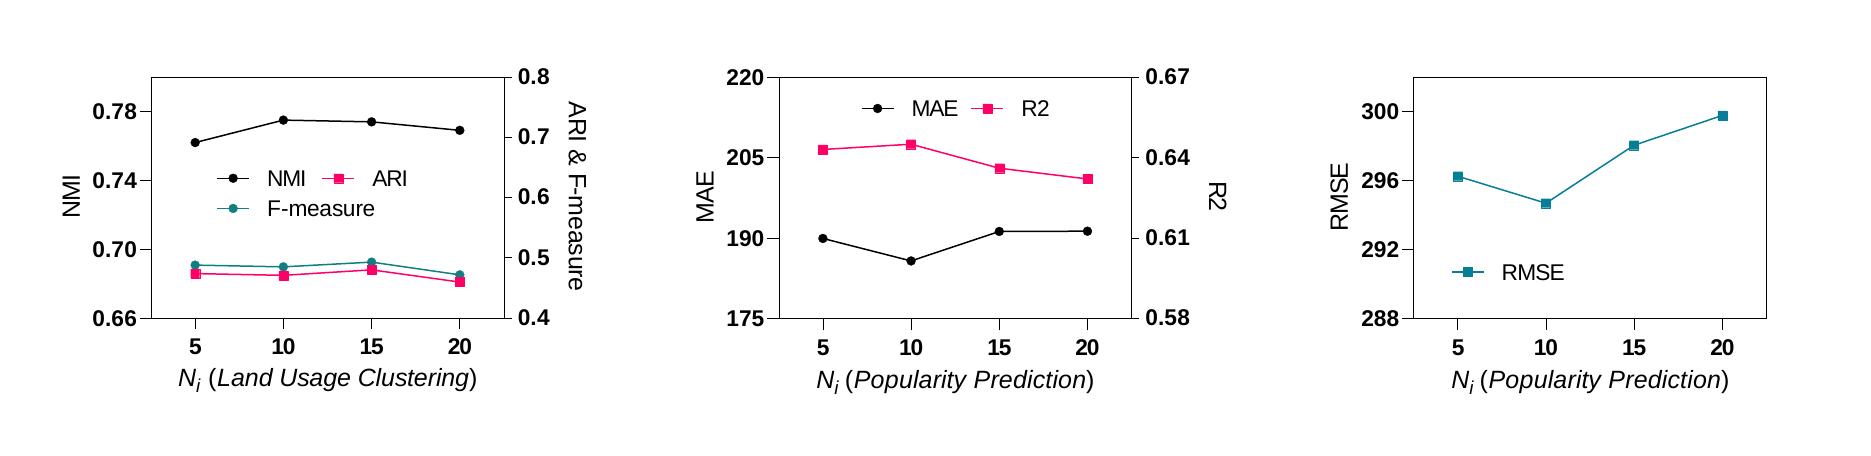}
		\caption{Parameter $N_i$}
		\label{fig:ni}
	\end{subfigure}
	\caption{Impact of intra/inter view negative sizes.}
    \vspace{-0.2cm}
	\label{fig:neg_size_app}
\end{figure}

{\FinalOne
\textbf{The negative sizes for intra/inter views.} As can be seen in Fig. \ref{fig:neg_size_app}, the model performances tend to increase firstly and then drop when negative sizes are too large for both intra and inter views. However, the largest difference between various experimental settings is less than 2\% for NMI (land usage clustering task) and 4\% for $R^2$ (popularity prediction task), showing that our model is  quite robust against these hyper-parameters.
}
